# Supplementary material for: Conceptual 12M: Pushing Web-Scale Image-Text Pre-Training To Recognize Long-Tail Visual Concepts
Source: arXiv:2102.08981 source file (2021-03-30)
Supplement: Supplementary file 1 [file supp.tex]

%auto-ignore

\documentclass[final]{cvpr}

\usepackage{times}
\usepackage{epsfig}
\usepackage{graphicx}
\usepackage{amsmath}
\usepackage{amssymb}

\usepackage{latexsym}

\usepackage{xspace}
\usepackage{caption}
\usepackage{subcaption} 
\usepackage{cprotect}
\usepackage{hhline}
\usepackage{array}
\usepackage{float}
\usepackage{enumitem}

\usepackage[pagebackref=true,breaklinks=true,colorlinks,bookmarks=false]{hyperref}

\newif\ifdraft
\draftfalse

\input{macros}

\begin{document}

\title{Conceptual 12M: Pushing Web-Scale Image-Text Pre-Training \\To Recognize Long-Tail Visual Concepts\\Supplementary Material}

\author{Soravit Changpinyo, Piyush Sharma, Nan Ding, Radu Soricut\\
Google Research\\
{\tt\small schangpi,piyushsharma,dingnan,rsoricut@google.com}}

\maketitle

\appendix

\input{supp_broader}
\input{supp_data}
\input{supp_qual}
\input{supp_pretraining}
\input{supp_exp_setup}

{\small
\bibliography{arxiv_main}
\bibliographystyle{ieee_fullname}
}

\end{document}
